# Supplementary material for: Conformal Off-Policy Evaluation in Markov Decision Processes
Source: arXiv:2304.02574 source file (2023-09-19)
Supplement: Supplementary file 1 [file A.appendix.tex]

\appendix
\section{Appendix}
\subsection{Proofs}

\begin{definition}
A sequence of random variables $\{V_{i}\}_{i=1}^n$ are weighted exchangeable, with weights $\{w_{i}\}_{i=1}^n$, if the density $f$ of their joint distribution can be expressed as
\begin{equation}
    f_{V_1,\dots,V_n}\left(v_{1}, \ldots, v_{n}\right)=\prod_{i=1}^{n} w_{i}\left(v_{i}\right) g\left(v_{1}, \ldots, v_{n}\right),
\end{equation}
where  $g$ is a function that is \emph{permutation-independent}, \emph{i.e.}, it does not depend on the order of the inputs, that is $g\left(v_{\sigma(1)}, \ldots, v_{\sigma(n)}\right)=$ $g\left(v_{1}, \ldots, v_{n}\right)$ for any permutation $\sigma$ of $\{1,\dots, n\}$.
\end{definition}
Note also the following lemma that follows from the definition of $w$.
\begin{lemma} Consider $\left\{\left(X_{i}, Y_{i}\right)\right\}_{i=1}^{n} \stackrel{\text { i.i.d. }}{\sim} P_{X, Y}^{\pi^{b}}$ and $\left(X_{n+1}, Y_{n+1}\right) \sim P_{X, Y}^{\pi}$.  Let $Z_{i}\coloneqq \left(X_{i}, Y_{i}\right) \in \mathbb{R}^{d} \times \mathbb{R}, i=1, \ldots, n+1$. Then $Z_{1}, \ldots, Z_{n+1}$ are weighted exchangeable with weights $w_{i} \equiv 1$, $i \leq n$ and $w_{n+1}(X, Y)=(\mathrm{d} P_{X, Y}^{\pi} / \mathrm{d} P_{X, Y}^{\pi^{b}})(X, Y)$.
\end{lemma}
Recall now that
\begin{align*}
p_{i}^{w}(x, y)&:=\frac{w\left(X_{i}, Y_{i}\right)}{\sum_{j=1}^{n} w\left(X_{j}, Y_{j}\right)+w(x, y)},\\
p_{n+1}^{w}(x, y)&:=\frac{w\left(x,y\right)}{\sum_{j=1}^{n} w\left(X_{j}, Y_{j}\right)+w(x, y)}.
\end{align*}
Then we have the following proposition.
\begin{proposition}
Let $\datacal\coloneqq\left\{(X_i, Y_i)\right\}_{i=1}^n \stackrel{\text { i.i.d. }}{\sim} P_{X, Y}^{\pi^b}$ be the calibration data. For any score function $s:\mathbb{R}^d\times \mathbb{R}\to\mathbb{R}$, and any $\alpha \in(0,1)$, let $V_i\coloneqq s(X_i,Y_i)$ and define the conformal predictive interval at a point $x \in \mathbb{R}^d$ as \begin{equation}
    \hat{C}_n(x)\coloneqq\left\{y \in \mathbb{R}: s(x, y) \leq \quantile{1-\alpha}\left(\hat{F}_n^{x, y}\right)\right\},
\end{equation}
where $
\hat{F}_n^{x, y}:= \sum_{i=1}^{n} p_{i}^{w}(x, y) \delta_{V_{i}}+p_{n+1}^{w}(x, y) \delta_{\infty}$, with exact weights $w(x, y)$.
If $P^{\pi}(y|x)$ is absolutely continuous w.r.t. $P^{\pi^b}(y | x)$, then $\hat{C}_n$ satisfies 
\begin{equation}
    \mathbb{P}_{(X, Y) \sim P_{X, Y}^{\pi}}\left(Y \in \hat{C}_n(X)\right) \geq 1-\alpha.
\end{equation}
\end{proposition}
\begin{proof}
The proof is the same as in \cite[Proposition 4.1]{taufiq2022conformal}.
Assume for simplicity that $V_{1}, \ldots, V_{n+1}$ are distinct almost surely. We define $f$ as the joint distribution of the random variables $\left\{X_{i}, Y_{i}\right\}_{i=1}^{n+1}$. We also denote $E_{z}$ as the event of $\left\{Z_{1}, \ldots, Z_{n+1}\right\}$ $=\left\{z_{1}, \ldots, z_{n+1}\right\}$ and let $v_{i}=s\left(z_{i}\right)=s\left(x_{i}, y_{i}\right)$, then for each $i$ :
\begin{align*}
&\mathbb{P}\left\{V_{n+1} =v_{i} \mid E_{z}\right\}=\mathbb{P}\left\{Z_{n+1}=z_{i} \mid E_{z}\right\},\\
&=\frac{\sum_{\sigma: \sigma(n+1)=i} f\left(z_{\sigma(1)}, \ldots, z_{\sigma(n+1)}\right)}{\sum_{\sigma} f\left(z_{\sigma(1)}, \ldots, z_{\sigma(n+1)}\right)}
\end{align*}
Now using the fact that $Z_{1}, \ldots, Z_{n+1}$ are weighted exchangeable:
\begin{align*}
&\frac{\sum_{\sigma: \sigma(n+1)=i} f\left(z_{\sigma(1)}, \ldots, z_{\sigma(n+1)}\right)}{\sum_{\sigma} f\left(z_{\sigma(1)}, \ldots, z_{\sigma(n+1)}\right)}\\
& =\frac{\sum_{\sigma: \sigma(n+1)=i} \prod_{j=1}^{n+1} w_{j}\left(z_{\sigma(j)}\right) g\left(z_{\sigma(1)}, \ldots, z_{\sigma(n+1)}\right)}{\sum_{\sigma} \prod_{j=1}^{n+1} w_{j}\left(z_{\sigma(j)}\right) g\left(z_{\sigma(1)}, \ldots, z_{\sigma(n+1)}\right)} \\
& =\frac{w_{n+1}\left(z_{i}\right) g\left(z_{1}, \ldots, z_{n+1}\right)}{\sum_{j=1}^{n+1} w_{n+1}\left(z_{j}\right) g\left(z_{1}, \ldots, z_{n+1}\right)} \\
& =p_{i}^{w}\left(z_{n+1}\right).
\end{align*}
Note that we get some simplifications due to the weights defined in Lemma 1, \emph{i.e.} $w_{i} \equiv 1$ for $i \leq n$ and $w_{n+1}(x, y)=w(x, y)=(\mathrm{d} P_{X, Y}^{\pi} / \mathrm{d} P_{X, Y}^{\pi^{b}})(x, y)$. Next, just as in \cite{tibshirani2019conformal} we can view:
\[
V_{n+1}=v_{i} \mid E_{z} \sim \sum_{i=1}^{n+1} p_{i}^{w}\left(z_{n+1}\right) \delta_{v_{i}}
\]
which implies that:
\[
\mathbb{P}\left\{V_{n+1} \leq \quantile{1-\alpha}\left(\sum_{i=1}^{n+1} p_{i}^{w}\left(z_{n+1}\right) \delta_{v_{i}}\right) \mid E_{z}\right\} \geq 1-\alpha .
\]
This is equivalent to
\[
\mathbb{P}\left\{V_{n+1} \leq \quantile{1-\alpha}\left(\sum_{i=1}^{n+1} p_{i}^{w}\left(Z_{n+1}\right) \delta_{v_{i}}\right) \mid E_{z}\right\} \geq 1-\alpha,
\]
and, after marginalizing, one has
\[
\mathbb{P}\left\{V_{n+1} \leq \quantile{1-\alpha}\left(\sum_{i=1}^{n+1} p_{i}^{w}\left(Z_{n+1}\right) \delta_{v_{i}}\right)\right\} \geq 1-\alpha.
\]
\end{proof}
\textbf{Proposition 4.2.} Let $\hat{C}_n$ be the conformal predictive intervals obtained as in Proposition 4.1, with weights $w(x, y)$ replaced by approximate weights $\hat{w}(x, y)=\hat{w}\left(x, y ; \mathcal{D}_{t r}\right)$, where the training data, $\mathcal{D}_{t r}$, is fixed. Assume that $\hat{w}(x, y)$ satisfies $\left(\mathbb{E}_{(X, Y) \sim P_{X, Y}^{\pi^b}}\left[\hat{w}(X, Y)^r\right]\right)^{1 / r} \leq M_r<\infty$ for some $r \geq 2$. Define $\Delta_w$ as
$$
\begin{aligned}
& \Delta_w:=\frac{1}{2} \mathbb{E}_{(X, Y) \sim P_{X, Y}^{\pi^b}}|\hat{w}(X, Y)-w(X, Y)| . \\
& \text { Then, } \mathbb{P}_{(X, Y) \sim P_{X, Y}^{\pi^*}}\left(Y \in \hat{C}_n(X)\right) \geq 1-\alpha-\Delta_w .
\end{aligned}
$$
If, in addition, non-conformity scores $\left\{V_i\right\}_{i=1}^n$ have no ties almost surely, then we also have
$$
\mathbb{P}_{(X, Y) \sim P_{X, Y}^{\pi^*}}\left(Y \in \hat{C}_n(X)\right) \leq 1-\alpha+\Delta_w+c n^{1 / r-1},
$$
for some positive constant $c$ depending only on $M_r$ and $r$.

Before detailing the main proof, we introduce a preliminary result which will be used in the proof of Proposition 4.2.
\\\\
\textbf{Lemma A.3.} Let $\hat{w}(x, y)$ be an estimate of the weights $w(x, y)=\mathrm{d} P_{X, Y}^{\pi^{*}} / \mathrm{d} P_{X, Y}^{\pi^{b}}(x, y)$, and $\left(\mathbb{E}_{(X, Y) \sim P_{X, Y}^{\pi^{b}}}\left[\hat{w}(X, Y)^{r}\right]\right)^{1 / r} \leq M_{r}<\infty$ for some $r \geq 2$. Let $\left(X_{i}, Y_{i}\right) \stackrel{\text { i.i.d. }}{\sim} P_{X, Y}^{\pi^{b}}$ and $\mathcal{A}$ denote the event that
$$
\sum_{i=1}^{n} \hat{w}\left(X_{i}, Y_{i}\right) \leq n / 2 .
$$
Then,
$$
\mathbb{P}(\mathcal{A}) \leq \frac{c_{1} M_{r}^{2}}{n}
$$

where $c_{1}$ is an absolute constant, and the probability is taken over $\left\{X_{i}, Y_{i}\right\}_{i=1}^{n} \stackrel{\text { i.i.d. }}{\sim} P_{X, Y}^{\pi^{b}}$.
\\\\
\textit{proof of Lemma A.3} 

The condition $\mathbb{E}_{(X, Y) \sim P_{X, Y}^{\pi^{b}}}\left[\hat{w}(X, Y)^{r}\right]<\infty \Longrightarrow \mathbb{P}_{(X, Y) \sim P_{X, Y}^{\pi^{b}}}(\hat{w}(X, Y)<\infty)=1$ and $\mathbb{E}_{(X, Y) \sim P_{X, Y}^{\pi b}}[\hat{w}(X, Y)]<\infty$. WLOG assume $\mathbb{E}_{(X, Y) \sim P_{X, Y}^{\pi b}}[\hat{w}(X, Y)]=1$. Recall that $p_{i}^{\hat{w}}(x, y):=\frac{\hat{w}\left(X_{i}, Y_{i}\right)}{\sum_{i=1}^{n} \hat{w}\left(X_{i}, Y_{i}\right)+\hat{w}(x, y)}$, and therefore, $p_{i}^{\hat{w}}(x, y)$ are invariant to weight scaling. Since $\mathbb{E}_{\left(X_{i}, Y_{i}\right) \sim P_{X, Y}^{\pi b}}\left[\hat{w}\left(X_{i}, Y_{i}\right)\right]^{2} \leq M_{r}^{2}$ and $\mathbb{E}_{\left(X_{i}, Y_{i}\right) \sim P_{X, Y}^{\pi b}}\left(\hat{w}\left(X_{i}, Y_{i}\right)\right)=1$, using Chebyshev's inequality

\begin{align}
&\mathbb{P}\left(\sum_{i=1}^{n} \hat{w}\left(X_{i}, Y_{i}\right) \leq n / 2\right)\\ 
&=\mathbb{P}\left(\sum_{i=1}^{n}\left(\hat{w}\left(X_{i}, Y_{i}\right)-1\right) \leq-n / 2\right) \\
& \leq \mathbb{P}\left(\left|\sum_{i=1}^{n}\left(\hat{w}\left(X_{i}, Y_{i}\right)-1\right)\right| \geq n / 2\right) \\
& \leq \frac{4}{n^{2}} \mathbb{E}\left[\left(\sum_{i=1}^{n} \hat{w}\left(X_{i}, Y_{i}\right)-\mathbb{E}\left[\hat{w}\left(X_{i}, Y_{i}\right)\right]\right)^{2}\right] \\
& =\frac{4}{n^{2}}\left\{n \mathbb{E}\left|\hat{w}\left(X_{1}, Y_{1}\right)-\mathbb{E}\left[\hat{w}\left(X_{1}, Y_{1}\right)\right]\right|^{2}\right\} \\
& \leq \frac{16}{n^{2}} n \mathbb{E}\left|\hat{w}\left(X_{1}, Y_{1}\right)\right|^{2} \\
& \leq \frac{c_{1} M_{r}^{2}}{n}
\end{align}

where to get from (16) to (17) we use:

$$
\begin{aligned}
&\mathbb{E}\left|\hat{w}\left(X_{1}, Y_{1}\right)-\mathbb{E}\left[\hat{w}\left(X_{1}, Y_{1}\right)\right]\right|^{2}\\ 
& \leq 2 \mathbb{E}\left[\hat{w}\left(X_{1}, Y_{1}\right)^{2}+\mathbb{E}\left[\hat{w}\left(X_{1}, Y_{1}\right)\right]^{2}\right] \\
& \leq 4 \mathbb{E}\left[\hat{w}\left(X_{1}, Y_{1}\right)^{2}\right] .
\end{aligned}
$$

\textit{Proof of Proposition 4.2} The condition $\mathbb{E}_{(X, Y) \sim P_{X, Y}^{\pi^{b}}}\left[\hat{w}(X, Y)^{r}\right]<\infty \Longrightarrow \mathbb{P}_{(X, Y) \sim P_{X, Y}^{\pi^{b}}}(\hat{w}(X, Y)<\infty)=1$ and $\mathbb{E}_{(X, Y) \sim P_{X, Y}^{\pi^{b}}}[\hat{w}(X, Y)]<\infty$. WLOG assume $\mathbb{E}_{(X, Y) \sim P_{X, Y}^{\pi^{b}}}[\hat{w}(X, Y)]=1$. Let $\tilde{P}_{X, Y}^{\pi^{*}}$ be a probability measure with

$$
\mathrm{d} \tilde{P}_{X, Y}^{\pi^{*}}(x, y):=\hat{w}(x, y) \mathrm{d} P_{X, Y}^{\pi^{b}}(x, y)
$$

and $(\tilde{X}, \tilde{Y}) \sim \tilde{P}_{X, Y}^{\pi^{*}}$ that is independent of the data. By Hölder's inequality,

$$
\begin{aligned}
\mathbb{E}_{(\tilde{X}, \tilde{Y}) \sim \tilde{P}_{X, Y}^{\pi^{*}}}[\hat{w}(\tilde{X}, \tilde{Y})] & =\int_{\tilde{x}, \tilde{y}} \frac{\mathrm{d} \tilde{P}^{\pi^{*}}(\tilde{x}, \tilde{y})}{\mathrm{d} P^{\pi^{b}}(\tilde{x}, \tilde{y})} \mathrm{d} \tilde{P}^{\pi^{*}}(\tilde{x}, \tilde{y}) \\
& =\mathbb{E}_{(X, Y) \sim P_{X, Y}^{\pi^{b}}}\left[\hat{w}(X, Y)^{2}\right]\\
&\leq M_{r}^{2}<\infty
\end{aligned}
$$

Note using Proposition $4.1$ with $(\tilde{X}, \tilde{Y})$ denoting $\left(X_{n+1}, Y_{n+1}\right)$ for simplicity

$$
\begin{aligned}
&\mathbb{P}(\tilde{Y} \in \hat{C}(\tilde{X}, \tilde{Y})) \\
& \quad=\mathbb{E}_{P_{X, Y}^{\pi*}}\left[\mathbb{P}\left(s(\tilde{X}, \tilde{Y}) \leq \text { Quantile }_{1-\alpha}(\hat{F}(\tilde{X}, \tilde{Y})) \mid \mathcal{E}(\tilde{V})\right)\right]
\end{aligned}
$$

where $\hat{F}(\tilde{X}, \tilde{Y}) = \sum_{i=1}^{n} p_{i}^{\hat{w}}(\tilde{X}, \tilde{Y}) \delta_{V_{i}}+p_{n+1}^{\hat{w}}(\tilde{X}, \tilde{Y}) \delta_{\infty}$ and $\mathcal{E}(\tilde{V})$ denotes the unordered set of $V_{1}, \ldots, V_{n+1}$. Marginalising over $\left\{\left(X_{i}, Y_{i}\right)\right\}_{i=1}^{n}$, we obtain

$$
(15) \leq \mathbb{E}\left(1-\alpha+\max _{i \in[n+1]} p_{i}^{\hat{w}}(\tilde{X}, \tilde{Y})\right)
$$

where the expectation is over $\left\{\left(X_{i}, Y_{i}\right)\right\}_{i=1}^{n} \stackrel{\text { i.i.i. }}{\sim} P_{X, Y}^{\pi^{b}}$ and $(\tilde{X}, \tilde{Y}) \sim \tilde{P}_{X, Y}^{\pi^{*}}$. Let $\mathcal{A}$ denote the event that

$$
\sum_{i=1}^{n} \hat{w}\left(X_{i}, Y_{i}\right) \leq n / 2 .
$$

using Lemma A.3 and $\mathbb{E}[\hat{w}(\tilde{X}, \tilde{Y})] \leq M_{r}^{2}$, we get that

$$
\begin{aligned}
& \mathbb{E}\left[\max _{i \in[n+1]} p_{i}^{\hat{w}}(\tilde{X}, \tilde{Y})\right]=\mathbb{E}\left[\frac{\max \left\{\hat{w}(\tilde{X}, \tilde{Y}), \max _{i} \hat{w}\left(X_{i}, Y_{i}\right)\right\}}{\hat{w}(\tilde{X}, \tilde{Y})+\sum_{i=1}^{n} \hat{w}\left(X_{i}, Y_{i}\right)}\right] \\
& \leq \mathbb{E}\left[\frac{\max \left\{\hat{w}(\tilde{X}, \tilde{Y}), \max _{i} \hat{w}\left(X_{i}, Y_{i}\right)\right\}}{\hat{w}(\tilde{X}, \tilde{Y})+\sum_{i=1}^{n} \hat{w}\left(X_{i}, Y_{i}\right)} \mathbbm{1}_{\mathcal{A}^{C}}\right]+\mathbb{P}(\mathcal{A}) \\
& \leq \mathbb{E}\left[\frac{2 \max \left\{\hat{w}(\tilde{X}, \tilde{Y}), \max _{i} \hat{w}\left(X_{i}, Y_{i}\right)\right\}^{n}}{n} \mathbbm{1}_{\mathcal{A}^{C}}\right]+\frac{c_{1} M_{r}^{2}}{n} \\
& \leq \frac{2}{n}\left(\mathbb{E}[\hat{w}(\tilde{X}, \tilde{Y})]+\mathbb{E} \max _{i} \hat{w}\left(X_{i}, Y_{i}\right)\right)+\frac{c_{1} M_{r}^{2}}{n} \\
& \leq \frac{2}{n}\left(\mathbb{E}[\hat{w}(\tilde{X}, \tilde{Y})]+\left(\sum_{i=1}^{n} \mathbb{E}\left[\hat{w}\left(X_{i}, Y_{i}\right)^{r}\right]\right)^{1 / r}\right)+\frac{c_{1} M_{r}^{2}}{n} \\
& \leq \frac{2}{n}\left(M_{r}^{2}+n^{1 / r} M_{r}\right)+\frac{c_{1} M_{r}^{2}}{n} .
\end{aligned}
$$

This implies that

$$
\mathbb{P}_{(X, Y) \sim \tilde{P}_{X, Y}^{\pi^{*}}}(Y \in \hat{C}(X)) \leq 1-\alpha+c n^{1 / r-1}
$$

for some constant $c$ that only depends on $M_{r}$ and $r$. Note that

\begin{align}
\left|\mathbb{P}_{\tilde{P}_{X, Y}^{\pi^{*}}}(Y \in \hat{C}(X))-\mathbb{P}_{P_{X, Y}^{\pi^{*}}}(Y \in \hat{C}(X))\right| \leq d_{\mathrm{TV}}\left(\tilde{P}^{\pi^{*}}, P^{\pi^{*}}\right)
\end{align}

where $d_{\mathrm{TV}}$ is the total variation norm which satisfies

\begin{align}
&d_{\mathrm{TV}}\left(\tilde{P}^{\pi^{*}}, P^{\pi^{*}}\right)\\
& =\frac{1}{2} \int\left|\hat{w}(x, y) \mathrm{d} P^{\pi^{b}}(x, y)-\mathrm{d} P^{\pi^{*}}(x, y)\right| \\
& =\frac{1}{2} \int\left|\hat{w}(x, y) \mathrm{d} P^{\pi^{b}}(x, y)-w(x, y) \mathrm{d} P^{\pi^{b}}(x, y)\right| \\
& =\frac{1}{2} \mathbb{E}_{(X, Y) \sim P_{X, Y}^{\pi^{b}}}[|\hat{w}(X, Y)-w(X, Y)|]=\Delta_{w}
\end{align}

Putting together (19) and (23), we get

$$
\mathbb{P}_{(X, Y) \sim P_{X, Y}^{\pi^{*}}}(Y \in \hat{C}(X)) \leq 1-\alpha+\Delta_{w}+c n^{1 / r-1}
$$

For the lower bound, using Proposition $4.1$ we get that

$$
\begin{aligned}
& \mathbb{P}_{(\tilde{X}, \tilde{Y}) \sim \tilde{P}_{X, Y}^{\pi^\ast}}(\tilde{Y} \in \hat{C}(\tilde{X}, \tilde{Y}))\\
&=\mathbb{P}\left(s(\tilde{X}, \tilde{Y}) \leq \operatorname{Quantile~}_{1-\alpha}(\hat{F})\right) \geq 1-\alpha .
\end{aligned}
$$

Using (19) we thus obtain

$$
\begin{aligned}
&\mathbb{P}_{(X, Y) \sim P_{X, Y}^{\pi^{*}}}(Y \in \hat{C}(X)) \\
& \geq \mathbb{P}_{(X, Y) \sim \tilde{P}_{X, Y}^{\pi^{*}}}(Y \in \hat{C}(X))-d_{T V}\left(\tilde{P}^{\pi^{*}}, P^{\pi^{*}}\right) \\
& \geq 1-\alpha-\Delta_{w}
\end{aligned}
$$
